# Supplementary material for: Dynamically inflated wind models of classical Wolf-Rayet stars
Source: arXiv:2012.05823 source file (2020-12-10)
Supplement: Supplementary file 1 [file Appendixes.tex]

%%%%%%%%   beginning of the appendixes  %%%%%%%%%%%%%
\begin{appendix}

\jon{NOTE: These below appendices still need to be either further developed (and significantly polished), or saved for Luka's PhD thesis. So no need for e.g. you Dylan or Stan to worry about them for now.}

\section{Thompson scattering atmosphere}\label{Ap_analitic_thompson}

In a case of the pure Thompson scattering atmosphere (e.i. constant Eddington ratio throughout the wind outflow) the formalism developed in the paper is reduced to the semi-analytic case in a steady-state approximation. Similar to Sec. \ref{Se_steady_state_dynamic_inflation} but now setting 
$\Gamma_{tot} = const > 1$ we can solve Eq. \ref{Eq_Lucy},\ref{Eq_motion_simp} considering supersonic limit when $a^2/v^2 \ll 1$. Under such assumptions we first arrive to:

\begin{equation}
v^2 = v_\infty^2\left(1 - \frac{R_c}{r}\right) + a_s^2\;,
\end{equation}
where used the inner boundary condition for velocity so that $v = a_s$ as $r = R_c$. The terminal velocity $v_\infty^2$ is now derived for $\Gamma_{tot} = const > 1$ law. Next, substituting $\kappa_{F} =  \Gamma_{tot}\kappa_e/\Gamma_e$ and density with Eq. \ref{Eq_massloos_rate}
we integrate Eq. \ref{Eq_tau_sp} using the outer boundary conditions to give us the optical depth at the inner boundary:

\begin{equation}\label{Eq_t_sp_cpnst_integra}
\tau_{sp}(R_c) = \frac{\Gamma_{tot} \kappa_e \dot M }{30\Gamma_e \pi R_c v_\infty}\left[8\left(1+\frac{a_s^2}{v_\infty^2}\right)^{5/2} -\right.
\end{equation}
 \[\left.-\frac{a_s}{v_\infty}\left(15 + 20\frac{a_s^2}{v_\infty^2} + 8\frac{a_s^4}{v_\infty^4}\right) \right]\;\]
using the fact that $a/v_\infty\ll1$ we simplify this to 
\begin{equation}
   \tau_{sp}(R_c) = \frac{4\Gamma_{tot} \kappa_e \dot M }{15\Gamma_e \pi R_c v_\infty} =  \frac{8}{15} \frac{\dot M v_\infty}{\L/c}\frac{\Gamma_{tot}}{\Gamma_{tot} - 1}
\end{equation}
Plugging this in Eq. \ref{Eq_Lucy} then gives the temperature at the inner boundary for a given $\Gamma_{tot}$ and assumed $\dot M$. 
Finally, to satisfy boundary conditions as descried in Sec. \ref{Se_steady_state_twopointer_boundary} to find self-consistent solution  the assumed $\dot M$ can be varied so that resulting $a_s$ and $\rho_s$ give $\Gamma_{OPAL}(a_s,\rho_s) = 1$. 

Alternatively, substitution of Eq. \ref{Eq_Lucy} with radiative diffusion Eq. \ref{Eq_static_prad} yields:

\[\frac{P_r}{P_g} = \frac{\L/c}{\dot M a_s}\tau_{sp}(R_c) = \frac{8}{15} \frac{ v_\infty}{ a_s }\frac{\Gamma_{tot}}{\Gamma_{tot} - 1}\]
or 
\begin{equation}
    P_g = \frac{15}{8}\frac{\Gamma_{tot} - 1}{v_\infty\Gamma_{tot}} \left(\frac{k_B}{\mu m_H}\right)^{1/2} \left(\frac{3 c }{4 \sigma_{SB} }\right)^{1/8} P_r^{9/8}
\end{equation}
with:
\[a_s = \sqrt[8]{\left(\frac{k_B}{\mu m_H}\right)^4\frac{3 c P_r}{4 \sigma_{SB} } }\]
This equation is now equivalent to Eq. 27 in \citet{Grafener_17} with the defence on ${15}/{8}$ factor that comes form there assumption that spherically modified optical depth can be replaced with  the  standard  Rosseland  mean  optical  depth Eq. \ref{Eq_tau_ph}

\section{Iterative solution of two-pointed boundary value problem}\label{Apx_iterative}

Numerical solution of two-pointed boundary value problem imposed in Sec. \ref{Se_steady_state_twopointer_boundary} requires an iterative procedure. As mentioned in Sec. \ref{Se_steady_state_dynamic_inflation} the iterative scheme is based on  Runge-Kutta  integrations and consists of two nested 
loops, \textit{force loop} which is the inner most loop and \textit{mass loss loop} outer loop. The \textit{force loop} it used to iteratively compute the self-consistent radiation force and \textit{mass loss loop} is designed to solve the two-pointed boundary value problem. 

\subsection{Mass loss loop}
To solve the two pointed boundary value problem a two step procedure is used, where on first step an inside-out integration $R_c\rightarrow R_{max}$ is performed using \textit{force loop} followed by second step with outside-in integration optical depth $R_c\leftarrow R_{max}$ using the wind structure from the first step.

\textit{Inside-out integration.} This step starts with setting the boundary value temperature $T_0$, which also gives boundary velocity as $v_0^2 = a_0^2 = k_B T_0/(\mu m_H)$. At the initial computation, user specified value is used but later $T_0$ is updated at the end of the second step. 

From the boundary temperature in OPAL table we then locate the density $\rho_0$ at which $\Gamma_{OPAL}(a_0,\rho_0) = 1$, setting the mass-loss rate $\dot M = 4\pi R_c^2 \rho_0 v_0$. \textit{force loop} is then called to perform the integration, returning the resulting wind velocity $v_{io}$ and temperature $T_{io}$ structures. However, derived temperature may not satisfy the outer boundary condition, therefore the results of this step are used in the following step to compute temperature structure starting from $R_{max}$.

\textit{Outside-in integration.} From Wind structure found on the prior step the spherically modified optical dept $\tau_{oi}$ defined by Eq. \ref{Eq_tau_sp} is computer starting at the outer boundary inwards. At the outer boundary optical depth $\tau_{out}$ is set as described in Sec.\ref{Se_steady_state_twopointer_boundary}. same way as it is done in Sec. \ref{Se_Time_dependant}. 
$\tau_{1}$ is computed from trapezoid integration and is used in  Eq. \ref{Eq_Lucy} to compute the temperature $T_{oi}$. As was the case with 
$T_{io}$ temperature computed on this step may not satisfy the inner boundary condition. If this is the case, then the $T_0$ is updated according to $\Delta_{T} = T_{io} - T_{oi}$ and both steps are repeated.

\textit{Convergence criterion.} In ideal case for the converged structure 
$\Delta_{T} = 0$. However at this is practically impossible we impose the convergence criterion $max(|\Delta_{T}|)\leq 3 [kK]$. Largest values of $\Delta_{T}$ are typically observable close to the outer boundary, but as discussed in Sec. \ref{Se_steady_state_dynamic_inflation} as the major part of the optical depth scale is accumulated in near inner boundary region even a difference of $3[kK]$ has only a moderate effect on setting the mass loss.

\subsection{Force loop} 
The force loop is designed to solve for self-consistent radiation force.
This loop is called within the \textit{Mass loss loop} and performs the integration to compute the wind velocity $v_{io}$ and temperature $T_{io}$ structure. integration is performed starting from inside boundary $R_c$ toward $R_{max}$. At the inner boundary velocity gradient $\d v\d r$ is computed using L’H\^opital’s rule by taking the numerical gradient of the OPAL table $\delta\Gamma_{OPAL}/\delta T|_{\rho =cont}$ and $\delta\Gamma_{OPAL}/\delta \rho|_{T =cont}$.
Starting with the inner boundary velocity gradient integration is performed using an explicit Runge-Kutta (4,5) based solver. actuale  \textit{force loop}, which allows to solve for self-consistent radiation force.
For convenience we integrate Eq. \ref{Eq_motion_simp} and differential form of Eq. \ref{Eq_Lucy} reformulated for square of sound speed:

\[ \frac{\d a^2}{\d r}= -\frac{k_{B}^4T_{c,\;eff}^4}{4\mu^4 m_h^4 a^6 }\left[\frac{R_c^2}{2r^3}\left(1 - \frac{R_c^2}{r^2}\right)^{-1/2} + \frac{3}{16\pi}\frac{\Gamma_{tot}\kappa_e \dot M R_c^2}{\Gamma_e r^4 v}\right]\]
temperature is then computed as $T_{io} = \mu m_H a^2/k_{B}$. 

This loop is required as the $\Gamma_{CAK,\; i}$  explicitly depends on the local velocity gradient $v\prime_i$, but integration scheme described earlier requires $v\prime_i$ at a given radial point, the $i$ here is used for a spacial indexing.  In tern,computation of velocity gradient requires knowledge of $\Gamma_{tot,\; i} = \Gamma_{OPAL,\; i} + \Gamma_{CAK,\; i}$ at the same point. To resolve this issue iterative procedure is applied where we use velocity gradient from prior iteration $^{n-1}v\prime_i$ to compute $^{n}\Gamma_{tot,\; i} = ^{n-1}\Gamma_{CAK,\;} +  ^{n}\Gamma_{OPAL,\; i}$, the $n$ is the iteration counter. At the end of each $^{n}\Gamma_{tot,\;i}$ is updated with $^{n}\Gamma_{CAK,\;}$.
Resulting current iteration wind structure is then compared to prior step and iteration is kept until the convergence criterion is met, at which point structure with self-consistent radiation force is found. To start of iterations, initially assumed initial velocity is used to compute the first $^0\Gamma_{tot,\;i}$. 

$\Gamma_{tot,\;i}$ is computed using exactly the same expression as in out time dependant numerical.
% model Eq. \ref{Eq_cak_g_discrete} in our time dependant simulation 

\textit{Convergence criterion} At the end of every iteration iteration errors $^{n}\Delta_{\Gamma} = ^{n-1}\Gamma_{tot} - ^{n}\Gamma_{tot}$, $^{n}\Delta_{v}= ^{n-1}v - ^{n}v$ and $^{n}\Delta_{T}= ^{n-1}T - ^{n}T$ are computed, which are used to 
\end{appendix}
